# Supplementary material for: Parameter Efficient Multi-task Model Fusion with Partial Linearization
Source: arXiv:2310.04742 source file (2024-03-11)
Supplement: Supplementary file 1 [file appendix.tex]

\documentclass{article} %
\usepackage{iclr2024_conference,times}

\input{math_commands.tex}

\usepackage[T1]{fontenc}

\definecolor{CColor}{rgb}{0.01,0.31,0.59}
\definecolor{GGray}{rgb}{0.80,0.90,1}
\definecolor{Shady}{rgb}{0.9,0.9,0.9}
\definecolor{kaistblue}{RGB}{20,135,200}
\definecolor{kaistdarkblue}{RGB}{0,65,145}
\definecolor{urbanablue}{RGB}{19,41,75}
\definecolor{urbanaorange}{RGB}{232,74,39}
\definecolor{drp}{rgb}{0.53,0.15,0.34}
\usepackage[plainpages=false,pdfpagelabels,colorlinks=true,linkcolor=CColor,citecolor=CColor,urlcolor=CColor]{hyperref}
\usepackage{url}
\usepackage{graphicx}
\usepackage{caption}
\usepackage{subcaption}
\usepackage{listings}
\usepackage{multirow}
\usepackage{bbold}

\lstdefinestyle{Python}{
    language=Python,
    basicstyle=\ttfamily\tiny,
    keywordstyle=\color{blue},
    stringstyle=\color{red!40!green},
    commentstyle=\color{brown},
    morekeywords={True, False},
    breakatwhitespace=false,
    breaklines=true,
    keepspaces=true,
    showstringspaces=false,
    showtabs=false
}

\newif\ifcameraready
\camerareadyfalse

\begin{document}

\appendix

\input{section/appendixA_experimental_details}
\input{section/appendixB_multitask_mf}

\clearpage
\input{section/appendixC_implementation}

\end{document}
